# Supplementary material for: A stable added-mass partitioned (AMP) algorithm for elastic solids and incompressible flow: model problem analysis
Source: arXiv:1812.03192 source file (2018-12-07)
Supplement: Supplementary file 1 [file analysisAppendix.tex]

\section{Stability analysis details} \label{sec:StabilityAnalysisDetails}

\subsection{CFL region for Cauchy scheme} \label{sec:CFLRegionCauchy}

In this section, stable CFL regions are derived for the solid discretizations in 
Sections~\ref{sec:viscousAnalysis} and~\ref{sec:inviscidAnalysis} applied to the 
pure initial-value problem (Cauchy problem). 
For both cases, we assume the spacial eigenfunction is given by $\phi=e\sp{i\vartheta}$
for all $\vartheta\in[0,2\pi].$
We define the CFL stability region as the region in the $\lx$-$\ly$ plane where $|A|\le 1.$
For a range of values in the
$\lx-\ly$ plane, the maximum amplification factor over $\vartheta\in[0,2\pi].$
was computed numerically to determine the region where $|A| \le 1.$ 
Figure~\ref{fig:viscousCFL} shows results for
equation~\eqref{eq:SolidDetCond} in Section~\ref{sec:viscousAnalysis} and
Figure~\ref{fig:inviscidCFL} shows results for
equation~\eqref{eq:evProblem} for Section~\ref{sec:inviscidAnalysis}.

{
\newcommand{\figWidth}{6cm}
\begin{figure}[h]
\begin{center}
\includegraphics[width=\figWidth]{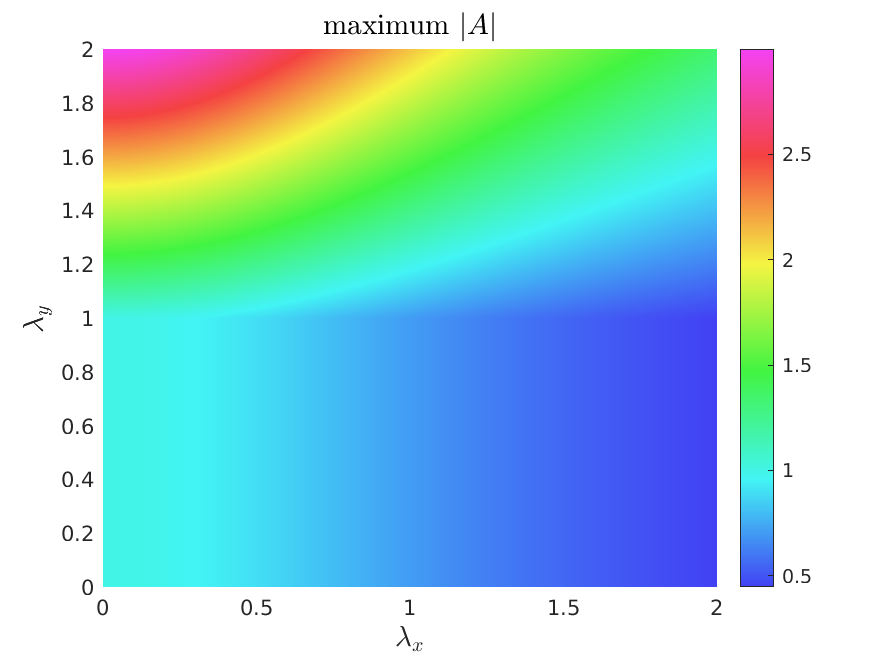}
\includegraphics[width=\figWidth]{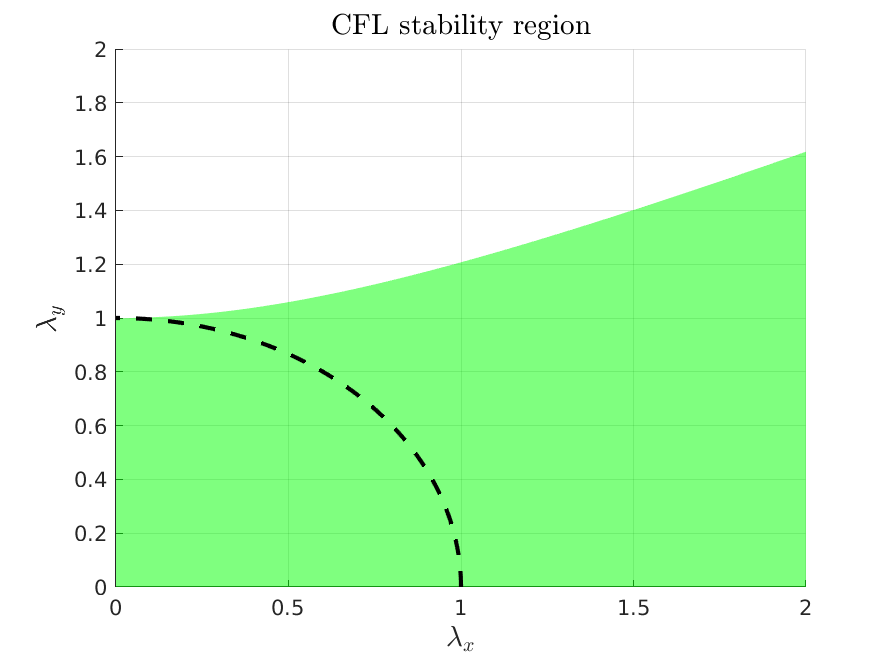}
\caption{Result for Section~\ref{sec:viscousAnalysis}.
Left: surface plot of the maximum amplification factor, $|A|$
over $\omega \in [0,2 \pi]$ for the Cauchy problem. 
Right: the green fill indicates the stability region $|A| \le 1.$ 
The dotted line represents the curve $\lx^2 + \ly^2 = 1,$ which is contained in 
the region. \label{fig:viscousCFL}}
\end{center}
\end{figure}

\begin{figure}[h]
\begin{center}
\includegraphics[width=\figWidth]{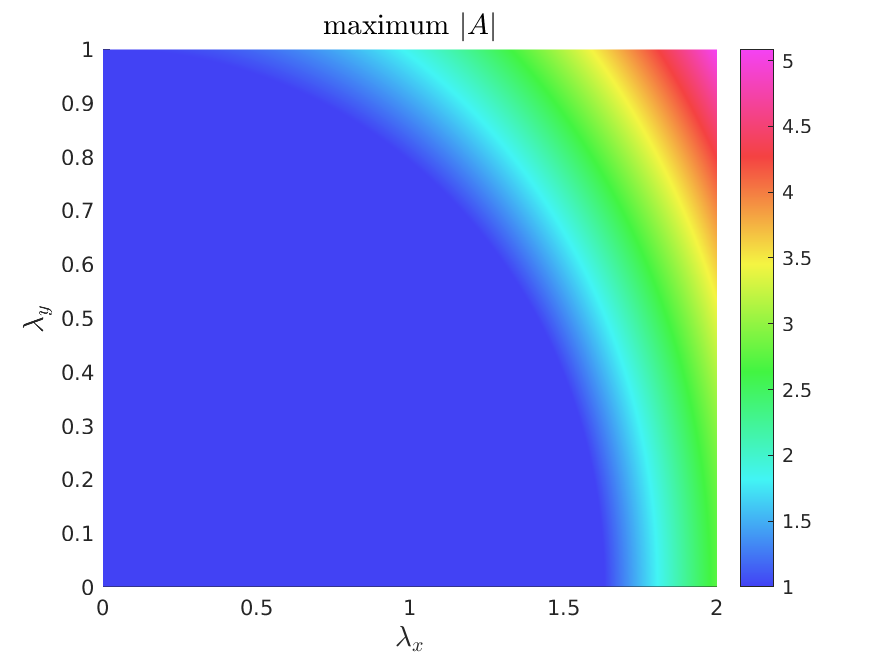}
\includegraphics[width=\figWidth]{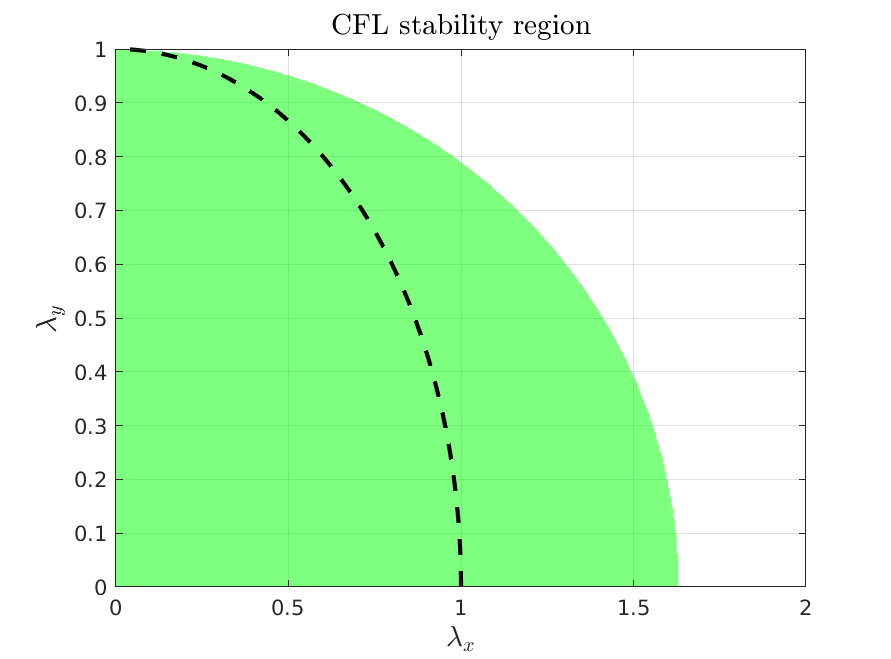}
\caption{Result for Section~\ref{sec:inviscidAnalysis}.
Left: surface plot of the maximum amplification factor, $|A|$
over $\omega \in [0,2 \pi]$ for the Cauchy problem. 
Right: the green fill indicates the stability region $|A| \le 1.$ 
The dotted line represents the curve $\lx^2 + \ly^2 = 1,$ which is contained in 
the region. \label{fig:inviscidCFL}}
\end{center}
\end{figure}
}
\subsection{Components of $\dMat$ for the viscous analysis} \label{sec:ComponentsOfDmatViscous}

Equation~\eqref{eq:StabilitySystemViscous} represents the system of equations that
arise when analyzing the stability of the MP-VA model problem.
The components of $\dMat$ can be obtained by substituting the solution to the discretization
into the incoming characteristic boundary conditions~\eqref{eq:a1CharBoundary}--\eqref{eq:a2CharBoundary}.
%%%%%%%%%%% {\it etaB} -> \eta(1/\phi)
%%%%%%%%%%% {\it etaA} -> \eta(\phi)
%%%%%%%%%%% {\it lx} -> \lx
%%%%%%%%%%% {\it ly} -> \ly
%%%%%%%%%%% etaA_:=1-A+ly*(phi-1): etaB_:=1-A+ly*(1/phi-1):
%%%%%%%%%%%
For the fully-coupled AMP scheme, the components are given by
\bse
\begin{align*}
g_{11} &= 2i (\phi-1) \eta(1/\phi) \mathcal{C} \\
g_{12} &= g_{21} = 0,\\
g_{22} &= -2 \lx A (\phi-1) \mathcal{C}.
\end{align*}
\ese
where
\begin{align*}
\mathcal{C} = \gamma^3 Z^2 + \gamma^2 Z^2 + \gamma^2 Z + 3 \gamma Z^2 + 2 \gamma Z - Z^2 + Z + 1.
\end{align*}
% old
% \bse
% \begin{align*}
% g_{11} &= { {2\,i \left( \phi-1 \right) \eta(1/\phi)\, \left( {\gamma}^{3}+{
% \gamma}^{2}+3\,\gamma-1 \right) {Z}^{2}+2\,i \left( \gamma+1 \right) ^
% {2} \left( \phi-1 \right) \eta(1/\phi)\,Z+2\,i \left( \phi-1 \right) \eta(1/\phi)}},\\
% g_{12} &= g_{21} = 0,\\
% g_{22} &= { {-2\,\lx\, \left( \phi-1 \right)  \left( {\gamma}^{3}+{
% \gamma}^{2}+3\,\gamma-1 \right) A{Z}^{2}-2\, \left( \gamma+1 \right) ^
% {2} \left( \phi-1 \right) A\lx\,Z-2\,\lx\, \left( \phi-1
%  \right) A}}.
% \end{align*}
% \ese
%
The components for the fractional-step AMP scheme are 
\begin{align*}
g_{11} &= 2 i (\phi-1) \eta(1/\phi) \mathcal{C}
\\
g_{12} &= g_{21} = 0
\\
g_{22} &= -2 \lx A (\phi-1) \mathcal{C}
\end{align*}
where
\begin{align*}
\mathcal{C} =\;&
4\, \left( \Lambda+1/2 \right)  \left( -1+ \left( \gamma+1 \right) 
 \left( \Lambda+1/2 \right) \gamma\,{A}^{2}-1/2\, \left( \gamma-1
 \right)  \left( \gamma+2\,\Lambda+2 \right) A \right) {Z}^{3}\\
&+A
 \left(  \left( \gamma+1 \right)  \left( 1+2\,{\Lambda}^{2}+ \left( 
\gamma+3 \right) \Lambda \right) A+ \left( -4\,{\gamma}^{2}-4\,\gamma
 \right) {\Lambda}^{3}+ \left( -2\,{\gamma}^{2}-2\,\gamma \right) {
\Lambda}^{2}-2\,\Lambda\,\gamma-\gamma-1 \right) {Z}^{2} \\
&+ \left( 
 \left( \gamma+1 \right) {A}^{2}-2\, \left( 1+\Lambda\, \left( \gamma+
1 \right)  \right)  \left( \Lambda+1/2 \right) A+2\,\Lambda+1 \right) 
\Lambda\,Z-A{\Lambda}^{2}.
\end{align*}
The components for the fractional-step TP scheme are 
\begin{align*}
g_{11} &= { {-i \left( 2\,ZA\lx-2\,\eta(1/\phi)\,\phi+\eta(1/\phi)
 \right) \Lambda-iZ \left( A-1 \right) \lx}}\\
g_{12} &= { {2\,iZ \left( A\Lambda+A/2-1/2 \right) \lx-i\eta(\phi)\,
\Lambda}}\\
g_{21} &= { {-Z\lx\, \left( \Lambda+1 \right)  \left( \gamma+1
 \right) {A}^{2}+ \left(  \left( \gamma+1 \right)  \left( -\gamma\,
\Lambda\,\eta(1/\phi)+\lx \right) Z-\lx\,\Lambda \right) A-2\,
\Lambda\,Z\eta(1/\phi)}}\\
g_{22} &= { {Z\lx\, \left( \Lambda+1 \right)  \left( \gamma+1 \right) 
{A}^{2}+ \left(  \left(  \left( -\gamma-1 \right) Z+ \left( -2\,\phi+1
 \right) \Lambda \right) \lx-Z\eta(\phi)\,\gamma\,\Lambda\,
 \left( \gamma+1 \right)  \right) A-2\,\Lambda\,Z\eta(\phi)}}
\end{align*}
The components for the fractional-step ATP scheme are 
\begin{align*}
  g_{11} &=   
           \big{(}
           2\,iZ \left( \phi-1/2 \right) \eta(1/\phi)\,{\gamma}^{3}+2\,i \left( 1/2+ \left( \phi-1/2 \right) Z \right) \eta(1/\phi)\,{\gamma}^{2} 
           + \left( i \left( 2\,Z\phi-Z+1 \right) \eta(1/\phi)+i\lx
           \right) \gamma \\ 
  &\phantom{= \big{(} }
  +2\,iZ \left( \phi-1/2 \right) \eta(1/\phi)-i\lx
           \big{)} A
           +4\,iZ \left( \phi-1/2 \right) \eta(1/\phi)\, \left( \gamma-1\right) \\
  g_{12} &= { { \left( i\eta(\phi)\,Z{\gamma}^{3}+i\eta(\phi)\, \left( Z-1
           \right) {\gamma}^{2}+i \left( \eta(\phi)\,Z-\eta(\phi)+\lx
           \right) \gamma+i \left( \eta(\phi)\,Z-\lx \right)  \right) A+2\,
           i\eta(\phi)\,Z \left( \gamma-1 \right) }}\\
  g_{21} &= { {\lx\,Z \left( \gamma+1 \right)  \left( {\gamma}^{2}+1
           \right) {A}^{2}+ \left(  \left(  \left( 2\,Z-1 \right) \lx-\eta(1/\phi) \right) \gamma+ \left( -2\,Z-1 \right) \lx-\eta(1/\phi)
           \right) A+2\,\eta(1/\phi)}}\\
  g_{22} &=  -2\,Z \left( {\gamma}^{2}+1 \right)  \left( \phi-1/2 \right) \lx\, \left( \gamma+1 \right) {A}^{2}+ \\
&\phantom{=}
  \left(  \left(  \left( -1+
           \left( -4\,\phi+2 \right) Z \right) \gamma-1
    + \left( 4\,\phi-2
           \right) Z \right) \lx+\eta(\phi)\, \left( \gamma+1 \right) 
           \right) A-2\,\eta(\phi)
\end{align*}

\subsection{Components of $\dMat$ for the inviscid analysis} \label{sec:ComponentsOfDmat}

Equation~\eqref{eq:StabilitySystem} represents the system of equations that
arise when analyzing the stability of the MP-IA model problem.
The components of $\dMat$ can be obtained by substituting the normal mode ansatz into
the solid boundary conditions (ie. equation~\eqref{eq:interfaceBCsForSolid}).
The first row of $\dMat$ is associated with boundary condition on the 
incoming characteristic.
For the AMP algorithm, the components of this row are given to be
\begin{align}
g_{1\nn, \;\text{AMP}} &= \frac{\beta_{2,\nn} M^2 + \beta_{1,\nn} M + \beta_{0,\nn} }
{\left(A^2 - \frac{4}{3} A + \frac{1}{3}\right) M^2
+ A^2 M + A^2} ,
\end{align}
where
\begin{align}
\beta_{0,\nn} &= A^2 \left(\qn{\nn} - \rn{\nn} - \qn{\nn} \left( \p_\nn + \frac{1}{\p_\nn} \right) \right),\\
\beta_{1,\nn} &= -A^2 \left( \frac{\qn{\nn}}{6} - \frac{5 \rn{\nn}}{6} 
+ \qn{\nn} \left(\p_\nn + \frac{1}{\p_\nn} \right)\right)
+ 2 A (\qn{\nn} - \rn{\nn})
+ \frac{1}{2} (\rn{\nn} - \qn{\nn}), \\
\beta_{2,\nn} &= \left(A^2 - \frac{4}{3} A + \frac{1}{3}\right)
\left(\qn{\nn} + \rn{\nn} - \qn{\nn} \left( \p_\nn + \frac{1}{\p_\nn}\right) \right) .
\end{align}
Similar expressions can be obtained for the TP and ATP algorithms. These expressions are 
given by
\begin{align}
\dComp_{1\nn, \;\text{TP}} &= 
(\rn{\nn} +\qn{\nn}) \left(\p_\nn + \frac{1}{\p_\nn} \right)
- M \frac{3A^2-4A+1}{A^2} (\rn{\nn}-\qn{\nn}),
\quad \nn=1,2, \\
\dComp_{1\nn, \;\text{ATP}} &= 
(\rn{\nn} -\qn{\nn}) \left(\p_\nn + \frac{1}{\p_\nn} \right)
- \frac{1}{4 M} \frac{A^2}{3A^2 - 4A + 1} (\rn{\nn} + \qn{\nn}),
\quad \nn=1,2.
\end{align}
The second row of 
$\dMat$ is common to all algorithms and represents 
extrapolation of the $\cp^+$ characteristic into the interface
ghost point. The second row is defined as
\begin{align}
\dComp_{2\nn} = \rn{\nn} \left(\p_\nn - 2 + \frac{1}{\p_\nn} \right), \quad \nn = 1,2.
\end{align}

\subsection{Exact solution for the 1D inviscid model problem} \label{sec:SolutionToOneDimensional}

In this section, we present an exact solution to the MP-IA model problem which is used
to verify the analytical stability regions.
Consider equations~\label{eq:solidModelDiscrete} in 1D ($k_x = 0$). 
The solution for the fluid pressure is given by
\begin{align}
p(y,t) = \rho \dot{v}_I(t) (H-y),
\end{align}
where $v_I(t)$ is the interface velocity.
In the solid, assume we are given the following initial conditions.
\begin{align}
a(y,0) = a_0(y), \quad b(y,0) = b_0(y)
\end{align}
The solution in the solid can be written as
\begin{align}
a(y,t) &= 
\begin{cases}
a_0(y+\cp t), & 0 < t < - y/\cp\\
a_I(t+y/\cp), & t > -y/\cp 
\end{cases}, \\
 b(y,t) &= b_0(y-\cp t),
\end{align}
where $a_I$ is the interface characteristic.
Since $b_I(t)$ is known for all time, we can use its definition to
form an ODE for the interface velocity, given by
\begin{align}
b_I(t) = -\rho H \dot{v}_I - \zp v_I.
\end{align}
The solution for the interface velocity is given by
\begin{align}
v_I(t) &= -\frac{1}{\rho H} \int_0^t e^{\lambda (\tau - t)} b_I(\tau) \; d \tau
 + v_I(0) e^{-\lambda t}, \\
\lambda &= \frac{\zp}{\rho H}.
\end{align}
The incoming solid characteristic at the interface $a_I$ can now be obtained using
\begin{align}
a_I(t) = -\rho H\dot{v}_I  + \zp v_I.
\end{align}
