# Supplementary material for: A stable added-mass partitioned (AMP) algorithm for elastic solids and incompressible flow: model problem analysis
Source: arXiv:1812.03192 source file (2018-12-07)
Supplement: Supplementary file 2 [file analysisAppendix-old.tex]

\section{Stability analysis details} \label{sec:StabilityAnalysisDetails}

\subsection{CFL region for Cauchy scheme} \label{sec:CFLRegionCauchy}

\das{Equation \eqref{eq:evProblem}.
For a range of values in the
$\lx-\ly$ plane, the maximum amplification factor over $\omega \in [0,2\pi]$ 
was computed numerically to determine the region where $|A| \le 1.$ }

{
\newcommand{\figWidth}{8cm}
\begin{figure}[h]
\begin{center}
\includegraphics[width=\figWidth]{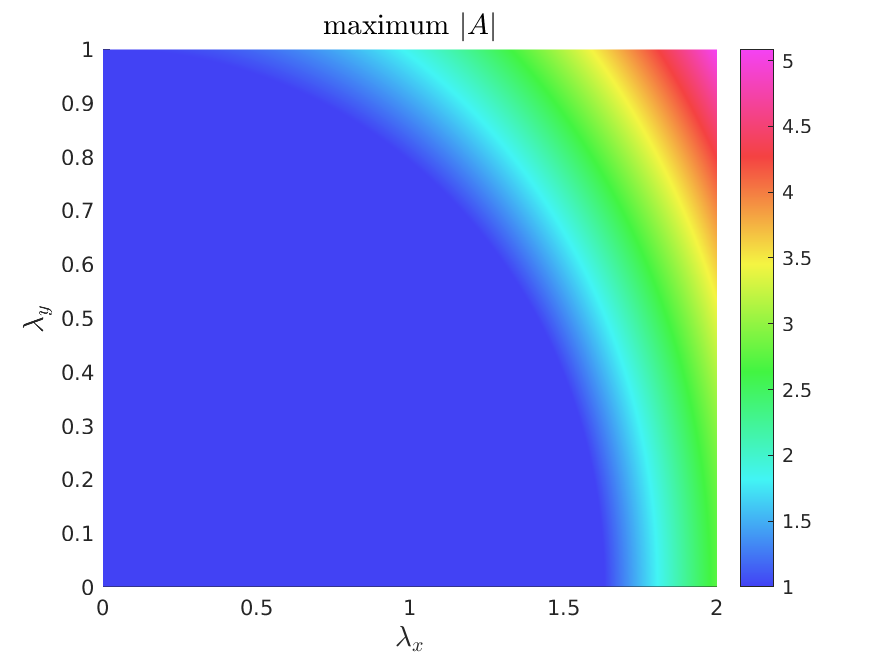}
\includegraphics[width=\figWidth]{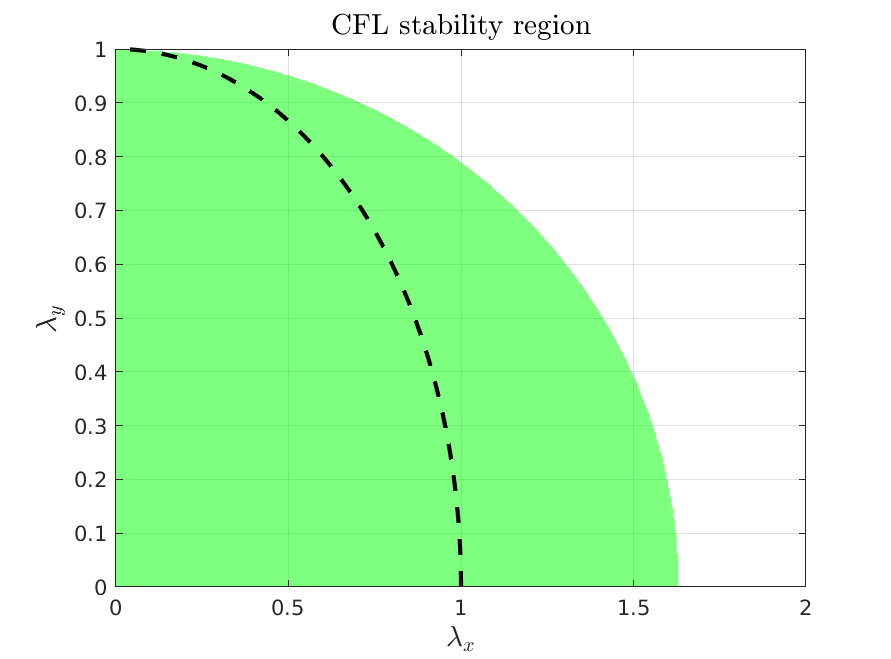}
\caption{Left: surface plot of the maximum amplification factor, $|A|$
over $\omega \in [0,2 \pi]$ for the Cauchy problem. 
Right: the green fill indicates the stability region $|A| \le 1.$ 
The dotted line represents the curve $\lx^2 + \ly^2 = 1,$ which is contained in 
the region.}
\end{center}
\end{figure}
}
\subsection{Components of $\dMat$} \label{sec:ComponentsOfDmat}

Equation \eqref{eq:StabilitySystem} represents the system of equations that
arise when analyzing the stability of the simplified model problem.
The components of $\dMat$ can be obtained by substituting the normal mode ansatz into
the solid boundary conditions (ie. equation \eqref{eq:interfaceBCsForSolid}).
The first row of $\dMat$ is associated with boundary condition on the 
incoming characteristic.
For the AMP algorithm, this components of this row are defined as
\begin{align}
g_{1\nn, \;\text{AMP}} &= \frac{\beta_{2,\nn} M^2 + \beta_{1,\nn} M + \beta_{0,\nn} }
{\left(A^2 - \frac{4}{3} A + \frac{1}{3}\right) M^2
+ A^2 M + A^2} ,
\end{align}
%
where
\begin{align}
\beta_{0,\nn} &= A^2 \left(\qn{\nn} - \rn{\nn} - \qn{\nn} \left( \p_\nn + \frac{1}{\p_\nn} \right) \right),\\
\beta_{1,\nn} &= -A^2 \left( \frac{\qn{\nn}}{6} - \frac{5 \rn{\nn}}{6} 
+ \qn{\nn} \left(\p_\nn + \frac{1}{\p_\nn} \right)\right)
+ 2 A (\qn{\nn} - \rn{\nn})
+ \frac{1}{2} (\rn{\nn} - \qn{\nn}), \\
\beta_{2,\nn} &= \left(A^2 - \frac{4}{3} A + \frac{1}{3}\right)
\left(\qn{\nn} + \rn{\nn} - \qn{\nn} \left( \p_\nn + \frac{1}{\p_\nn}\right) \right) .
\end{align}
%
Similar expressions can be obtained for the TP and ATP algorithms. These expressions are 
given by
\begin{align}
\dComp_{1\nn, \;\text{TP}} &= 
(\rn{\nn} +\qn{\nn}) \left(\p_\nn + \frac{1}{\p_\nn} \right)
- M \frac{3A^2-4A+1}{A^2} (\rn{\nn}-\qn{\nn}),
\quad \nn=1,2, \\
\dComp_{1\nn, \;\text{ATP}} &= 
(\rn{\nn} -\qn{\nn}) \left(\p_\nn + \frac{1}{\p_\nn} \right)
- \frac{1}{4 M} \frac{A^2}{3A^2 - 4A + 1} (\rn{\nn} + \qn{\nn}),
\quad \nn=1,2.
\end{align}
%
The second row of 
$\dMat$ is common to all algorithms and represents 
extrapolation of the $\cp^+$ characteristic into the interface
ghost point. The second row is defined as
\begin{align}
\dComp_{2\nn} = \rn{\nn} \left(\p_\nn - 2 + \frac{1}{\p_\nn} \right), \quad \nn = 1,2.
\end{align}
%



\subsection{Derivation of the piece-wise definition of $\p_1$ and $\p_2$
for the 1D analysis} \label{sec:PiecewiseDefinition}

Recall the definition of 
$\p_{\bc,\pm}$ and $\p_{\ac,\pm}$ in equation \eqref{eq:eigenvalueOneD}.
The discriminant of $\p_{\bc,\pm}$, $D$, is given by
\begin{align}
D = A^2 - (2 A - 1 ) (1-\ly^2).
\end{align}
% 
A branch cut discontinuity occurs when $D$ is on the negative real line
($\Re(D) < 0, \Im(D) = 0$).
Let $A = A_r + i A_i$. Upon substitution, the discriminant becomes
\begin{align}
D = A_r^2 - A_i^2 + (\ly^2 - 1) (2 A_r - 1)  
+ 2 i A_i \left( A_r + \ly^2 - 1 \right) .
\end{align}
%
The imaginary part of $D$ is zero when either $A_r = 1-\ly^2$ or $A_i = 0.$
We are interested in the behavior of the roots when $|A| > 1$
and $0 \le \ly \le 1.$ \\

%
\noindent \textbf{Case 1}: $A_r = 1-\ly^2.$ Since $|A| > 1,$ we must have
\begin{align}
A_i^2 > 1 - (1-\ly^2)^2. \label{eq:branchCutInequality}
\end{align}
%
Using this fact, we can show the following about the real part of $D$.
\begin{align}
\Re(D) = \ly^2 (1 - \ly^2) - A_i^2 
< \ly^2 (1- \ly^2) - 1 + (1-\ly^2)^2 
< -\ly^2
< 0
\end{align}
% 
Since $\Re(D) < 0,$ we have that there is a branch cut when $A_r = 1-\ly^2.$ \\

\noindent \textbf{Case 2}: $A_i = 0.$ 
% Since $|A| > 1,$ we must have
% \begin{align}
% A_r^2 > 1
% \end{align}
%
When this is true, we can show the following about the real part of $D$.
\begin{align}
\Re(D) = A_r^2 + (\ly^2 - 1) (2 A_r - 1)
= (A_r + (\ly^2 - 1))^2 + (1-\ly^2)\ly^2 > 0
\end{align}
%
Since $\Re(D) > 0,$ $A_i = 0$ is not a branch cut.

We have determined that there is a branch cut discontinuity 
along the line $A_r = 1 - \ly^2$ when $|A| > 1$ and $0 \le \ly \le 1$.
As shown in the lemma, $|\p_{\bc,\pm}| \ne 1$ when $|A| > 1.$
Due to continuity,
$\p_{\bc,+}$ cannot cross the unit circle, $|\p_{\bc,+}| = 1$, 
unless the branch cut is crossed. Therefore it is only necessary to 
check where $\p_{\bc,+}$ lies relative to the unit circle for a single point.
Let $A = 1 + \epsilon,$ for $\epsilon > 1.$
We can show that the (real-valued) numerator of $\p_{\bc,+}$ is 
greater than the denominator of $\p_{\bc,+}.$
\begin{align*}
A - (1-\ly^2) + \sqrt{A^2 - (2 A - 1) (1-\ly^2)}
&= \ly^2 + \epsilon + \sqrt{\ly^2 + 2 \epsilon \ly^2 + \epsilon^2}  > \ly^2 + \ly
\end{align*}
%
Because of this, $|\p_{\bc,+}| > 1$ when $A_r > 1-\ly^2.$
The final task is determining the size of $|\p_{\bc,+}|$ when 
$A_r = 1-\ly^2.$ In this case we can use
equation \eqref{eq:branchCutInequality} to bound the discriminant by
\begin{align}
D = \ly^2 (1-\ly^2) - A_i^2 < \ly^2 - \ly^4 - 2 \ly^2 + \ly^4 < - \ly^2.
\end{align}
%
This implies that
\begin{align}
\sqrt{D} = C i,
\end{align}
%
for some $C > \ly$.
Therefore we have that $\phi_{\bc}$ is purely imaginary on 
the branch cut, given by 
\begin{align}
\phi_{\bc,\pm} = i \frac{A_i \pm C }{\ly( \ly + 1)}.
\end{align}
%
$A_i$ can either be positive or negative as long as
equation \eqref{eq:branchCutInequality} is obeyed.
When $A_i > \ly \sqrt{2 - \ly^2}$, we have
\begin{align}
|\phi_{a,+}| > \frac{\ly \sqrt{2-\ly^2} + \ly}{\ly^2 + \ly} > 1.
\end{align}
%
On the other hand, when $A_i < -\ly \sqrt{2-\ly^2}$, we have
\begin{align}
|\phi_{a,-}| > \frac{\ly \sqrt{2-\ly^2} + \ly}{\ly^2 + \ly} > 1.
\end{align}
%
Using the condition in equation \eqref{eq:SizeOfEigenvalues}
from the lemma and the fact that
\begin{align}
\p_{\bc,\pm} = \frac{1}{\p_{b,\mp}},
\end{align}
%
we have
\begin{align}
\p_1 &= 
\begin{cases}
\p_{\bc,+}, & \Re(A) > 1 - \ly^2 \\
\p_{\bc,+}, & \Re(A) = 1 - \ly^2 \text{ and } \Im(A) > 0\\
\p_{\bc,-}, & \Re(A) < 1 - \ly^2 \\
\p_{\bc,-}, & \Re(A) = 1 - \ly^2 \text{ and } \Im(A) < 0
\end{cases} \\
\p_2 &= 
\begin{cases}
\p_{\ac,+}, & \Re(A) > 1 - \ly^2 \\
\p_{\ac,+}, & \Re(A) = 1 - \ly^2 \text{ and } \Im(A) > 0\\
\p_{\ac,-}, & \Re(A) < 1 - \ly^2 \\
\p_{\ac,-}, & \Re(A) = 1 - \ly^2 \text{ and } \Im(A) < 0
\end{cases} .
\end{align}


\subsection{Solution to 1D analysis problem} \label{sec:SolutionToOneDimensional}

\das{here are brief details. I'll expand this if we decide to include.}
In 1D, $k_x = 0$. The fluid pressure is given by
\begin{align}
p(y,t) = \rho \dot{v}_I(t) (H-y),
\end{align}
%
where $v_I(t)$ is the interface velocity.
In the solid we are given the following initial conditions
\begin{align}
a(y,0) = a_0(y), \quad b(y,0) = b_0(y).
\end{align}
%
The solution in the solid can be written as
\begin{align}
a(y,t) &= 
\begin{cases}
a_0(y+\cp t), & 0 < t < - y/\cp\\
a_I(t+y/\cp), & t > -y/\cp 
\end{cases}, \\
 b(y,t) &= b_0(y-\cp t),
\end{align}
% 
where $a_I$ is the interface characteristic.
Since $b_I(t)$ is known for all time, we can use its definition to
form an ODE for the interface velocity, given by
\begin{align}
b_I(t) = -\rho H \dot{v}_I - \zp v_I.
\end{align}
%
The solution is
\begin{align}
v_I(t) &= -\frac{1}{\rho H} \int_0^t e^{\lambda (\tau - t)} b_I(\tau) \; d \tau
 + v_I(0) e^{-\lambda t} \\
\lambda &= \frac{\zp}{\rho H}.
\end{align}
%
$a_I$ can now be obtained
\begin{align}
a_I(t) = -\rho H\dot{v}_I  + \zp v_I.
\end{align}
